# Supplementary material for: Regression Prior Networks
Source: arXiv:2006.11590 source file (2020-12-09)
Supplement: Supplementary file 1 [file leftovers.tex]

%\begin{figure}[ht!]
%\centering
%\includegraphics[scale=0.25]{figures/power_uncertainty.png}
%\caption{Comparison of unc measures on power dataset}\label{fig:unc_power}
%\end{figure}

%\begin{figure}[ht!]
%\centering
%\includegraphics[scale=0.25]{figures/msd_uncertainty.png}
%\caption{Comparison of unc measures on msd dataset}\label{fig:unc_msd}
%\end{figure}

% % RMSE and NLL 




% \begin{figure}[!ht]
% \centering
% \subfigure[{Nyu $\ln \mathbb{V}[y]$ - ID}]{
% \includegraphics[scale=0.131]{figures/nuy_plots/histograms/ID/log_total_variance_mean.png}}
% \subfigure[Nyu E. Ent - ID]{
% \includegraphics[scale=0.131]{figures/nuy_plots/histograms/ID/expected_entropy_mean.png}}
% \subfigure[{Nyu $\ln \mathbb{E}[\bm{\Sigma}]$ - ID}]{
% \includegraphics[scale=0.131]{figures/nuy_plots/histograms/ID/log_expected_variance_mean.png}}
% \subfigure[{Nyu $\ln \mathbb{V}[\bm{\mu}]$ - ID}]{
% \includegraphics[scale=0.131]{figures/nuy_plots/histograms/ID/log_variance_of_expected_mean.png}}
% \\
% \subfigure[{LSUN $\ln \mathbb{V}[y]$ - OOD}]{
% \includegraphics[scale=0.131]{figures/nuy_plots/histograms/OOD/log_total_variance_mean.png}}
% \subfigure[LSUN E. Ent - OOD]{
% \includegraphics[scale=0.131]{figures/nuy_plots/histograms/OOD/expected_entropy_mean.png}}
% \subfigure[{LSUN $\ln \mathbb{E}[\bm{\Sigma}]$ - OOD}]{
% \includegraphics[scale=0.131]{figures/nuy_plots/histograms/OOD/log_expected_variance_mean.png}}
% \subfigure[{LSUN $\ln \mathbb{V}[\bm{\mu}]$ - OOD}]{
% \includegraphics[scale=0.131]{figures/nuy_plots/histograms/OOD/log_variance_of_expected_mean.png}}
% \\
% \subfigure[{KITTI $\ln \mathbb{V}[y]$ - OOD}]{
% \includegraphics[scale=0.131]{figures/nuy_plots/histograms/OOD2/log_total_variance_mean.png}}
% \subfigure[KITTI E. Ent - OOD]{
% \includegraphics[scale=0.131]{figures/nuy_plots/histograms/OOD2/expected_entropy_mean.png}}
% \subfigure[{KITTI $\ln \mathbb{E}[\bm{\Sigma}]$ - OOD}]{
% \includegraphics[scale=0.131]{figures/nuy_plots/histograms/OOD2/log_expected_variance_mean.png}}
% \subfigure[{KITTI $\ln \mathbb{V}[\bm{\mu}]$ - OOD}]{
% \includegraphics[scale=0.131]{figures/nuy_plots/histograms/OOD2/log_variance_of_expected_mean.png}}

% \caption{Comparison of image-wise uncertainty measures between single model, ensemble and EnD$^2$.}\label{fig:nyu_unc_hists_mean}
% \end{figure}

% \begin{figure}[!ht]
% \centering
% \subfigure[{Nyu $\ln \mathbb{V}[y]$ - ID}]{
% \includegraphics[scale=0.131]{figures/nuy_plots/histograms/ID/log_total_variance_none.png}}
% \subfigure[Nyu E. Ent - ID]{
% \includegraphics[scale=0.131]{figures/nuy_plots/histograms/ID/expected_entropy_none.png}}
% \subfigure[{Nyu $\ln \mathbb{E}[\bm{\Sigma}]$ - ID}]{
% \includegraphics[scale=0.131]{figures/nuy_plots/histograms/ID/log_expected_variance_none.png}}
% \subfigure[{Nyu $\ln \mathbb{V}[\bm{\mu}]$ - ID}]{
% \includegraphics[scale=0.131]{figures/nuy_plots/histograms/ID/log_variance_of_expected_none.png}}
% \\
% \subfigure[{LSUN $\ln \mathbb{V}[y]$ - OOD}]{
% \includegraphics[scale=0.131]{figures/nuy_plots/histograms/OOD/log_total_variance_none.png}}
% \subfigure[LSUN E. Ent - OOD]{
% \includegraphics[scale=0.131]{figures/nuy_plots/histograms/OOD/expected_entropy_none.png}}
% \subfigure[{LSUN $\ln \mathbb{E}[\bm{\Sigma}]$ - OOD}]{
% \includegraphics[scale=0.131]{figures/nuy_plots/histograms/OOD/log_expected_variance_none.png}}
% \subfigure[{LSUN $\ln \mathbb{V}[\bm{\mu}]$ - OOD}]{
% \includegraphics[scale=0.131]{figures/nuy_plots/histograms/OOD/log_variance_of_expected_none.png}}
% \\
% \subfigure[{KITTI $\ln \mathbb{V}[y]$ - OOD}]{
% \includegraphics[scale=0.131]{figures/nuy_plots/histograms/OOD2/log_total_variance_none.png}}
% \subfigure[KITTI E. Ent - OOD]{
% \includegraphics[scale=0.131]{figures/nuy_plots/histograms/OOD2/expected_entropy_none.png}}
% \subfigure[{KITTI $\ln \mathbb{E}[\bm{\Sigma}]$ - OOD}]{
% \includegraphics[scale=0.131]{figures/nuy_plots/histograms/OOD2/log_expected_variance_none.png}}
% \subfigure[{KITTI $\ln \mathbb{V}[\bm{\mu}]$ - OOD}]{
% \includegraphics[scale=0.131]{figures/nuy_plots/histograms/OOD2/log_variance_of_expected_none.png}}

% \caption{Comparison of pixel-wise uncertainty measures between single model, ensemble and EnD$^2$.}\label{fig:nyu_unc_hists_none}
% \end{figure}
